# Supplementary material for: An Analytical Model for Performance and Lifetime Estimation of Hybrid DRAM-NVM Main Memories
Source: arXiv:1903.10067 source file (2019-03-24)
Supplement: Supplementary file 1 [file appendix.tex]

\documentclass[10pt,journal,compsoc]{IEEEtran}

\ifCLASSOPTIONcompsoc
% The IEEE Computer Society needs nocompress option
% requires cite.sty v4.0 or later (November 2003)
\usepackage[nocompress]{cite}
\else
% normal IEEE
\usepackage{cite}
\fi

\usepackage{graphicx}
\usepackage{soul}
\usepackage[linesnumbered,ruled]{algorithm2e}
\usepackage{subfig}
\usepackage[fleqn]{amsmath}
\usepackage{relsize}
% Vector notation
\usepackage{mathtools}

\usepackage{ragged2e}
\usepackage{booktabs} % For formal tables
\usepackage[percent]{overpic}
\usepackage{relsize}
\usepackage{multirow}
\usepackage{amssymb}
\usepackage{bm}
\usepackage{enumitem}
\usepackage{amsmath}
\usepackage[normalem]{ulem}
\usepackage{tikz}

\soulregister\cite7
\soulregister\ref7
\soulregister\pageref7

\begin{document}
	
\appendices

\newcommand{\textoverline}[1]{$\overline{\mbox{#1}}$}
\newcommand{\specialcell}[2][c]{%
	\begin{tabular}[#1]{@{}l@{}}#2\end{tabular}}

\vspace{-.3cm}
\section{HMA Assumptions}
\label{sec:hmaassumption}
In this section, the assumptions on HMAs that can be evaluated by the proposed analytical model are presented.
To accurately define the assumptions, a definition for HMAs is presented first.
Then based on this definition, the assumptions made for HMAs which enables us to accurately predict their behavior are provided.

\subsection{Hybrid memories definition}
%HMAs can employ a vast range of management policies either globally or per memory module.
%Modelling all hybrid memories requires very complex models which significantly increases the required computations that might be impractical in many cases.
%Therefore, to decrease the model complexity, a few restrictions are defined for the modelled hybrid memories.
%Considering such restrictions, the proposed analytical model is still able to cover a wide range of hybrid memories.
%To discuss the proposed model restrictions, a definition for hybrid memories is presented which is used for denoting model restrictions.
HMAs can be defined by a tuple denoted as \textless mapping, Upd, Mig, EvicP\textgreater\space which is detailed as follows:
\textbf{\emph{(a)}} \emph{mapping} stores required information for managing memory (per data page) such as position in LRU queue or reference and dirty bits alongside clock handle position in the Clock algorithm.
Two subsets of \emph{mapping} can also be presented to depict data pages residing in DRAM and NVM which are denoted as \emph{mapping.DRAM} and \emph{mapping.NVM}, respectively.
\textbf{\emph{(b)}} For each access to the memory subsystem, \emph{Upd(mapping, Page, \textoverline{NewMapping})}\footnote{Parameters with overline are outputs.} function will be called which reconfigures the internal placement of data pages (setting ref bit in Clock and moving the data page to the \emph{Most Recently Used} (MRU) position in queue in LRU algorithm).
\emph{Upd} function calls other functions to decide page replacements in case of migrations or free space shortage in memory.
\textbf{\emph{(c)}} Any required movement of data pages between memories are governed by \emph{Mig(mapping, \textoverline{MigPage})} function which decides whether or not a data page should be moved to another memory module.
\textbf{\emph{(d)}} In case of a miss access, \emph{EvicP(mapping, Page, \textoverline{Prob})} is called to calculate the eviction probability for data pages and deciding the data page which should be evicted from the memory.

\begin{figure*}[t]
	\centering
	\subfloat[blackscholes]{\includegraphics[width=0.242\textwidth]{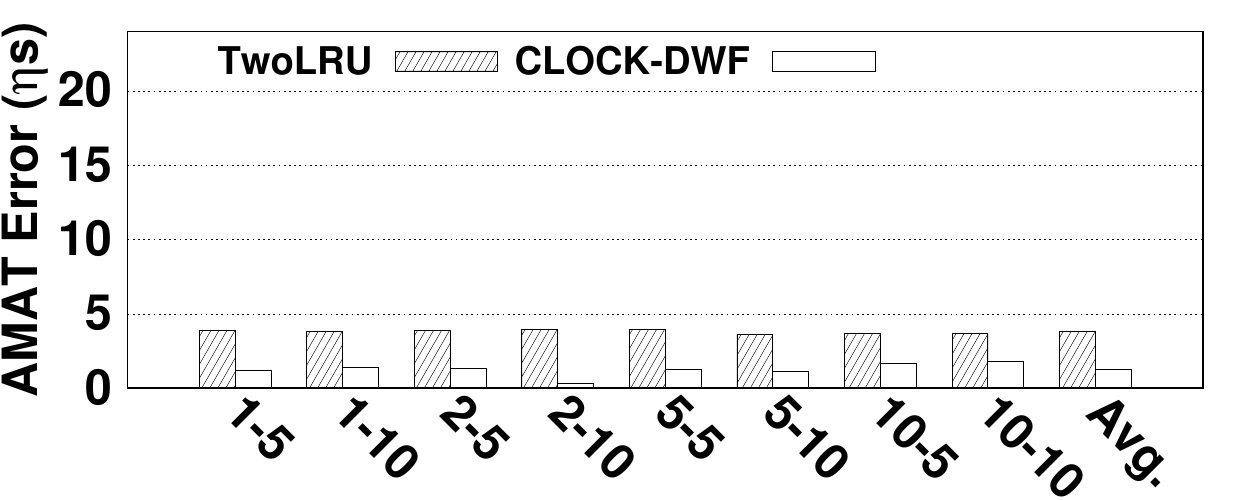}
		\label{fig:blackscholes-lifetime}}
	\hfill
	\subfloat[bodytrack]{\includegraphics[width=0.242\textwidth]{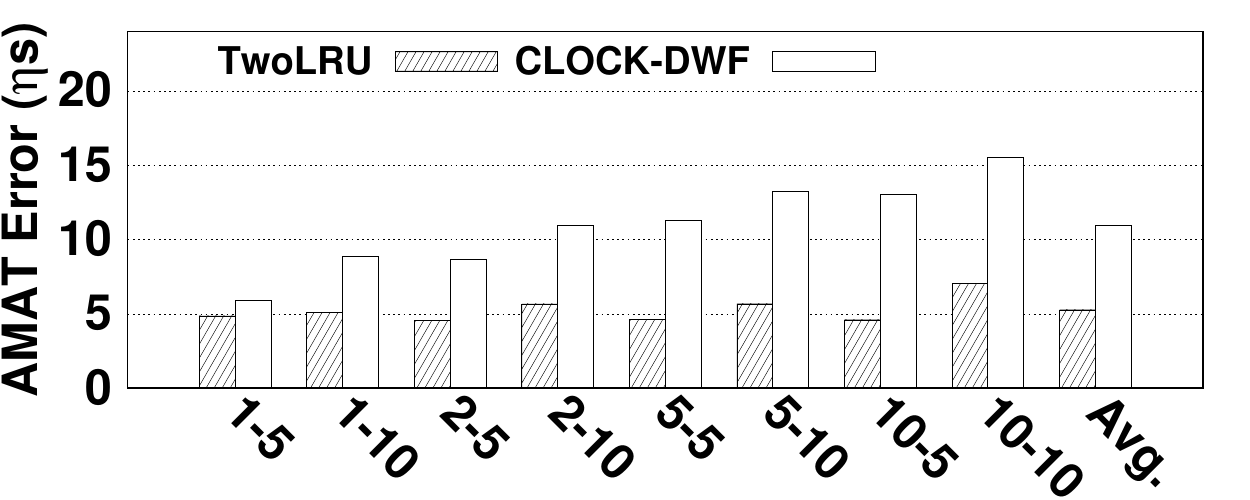}
		\label{fig:bodytrackerror-lifetime}}
	\hfill
	\subfloat[canneal]{\includegraphics[width=0.242\textwidth]{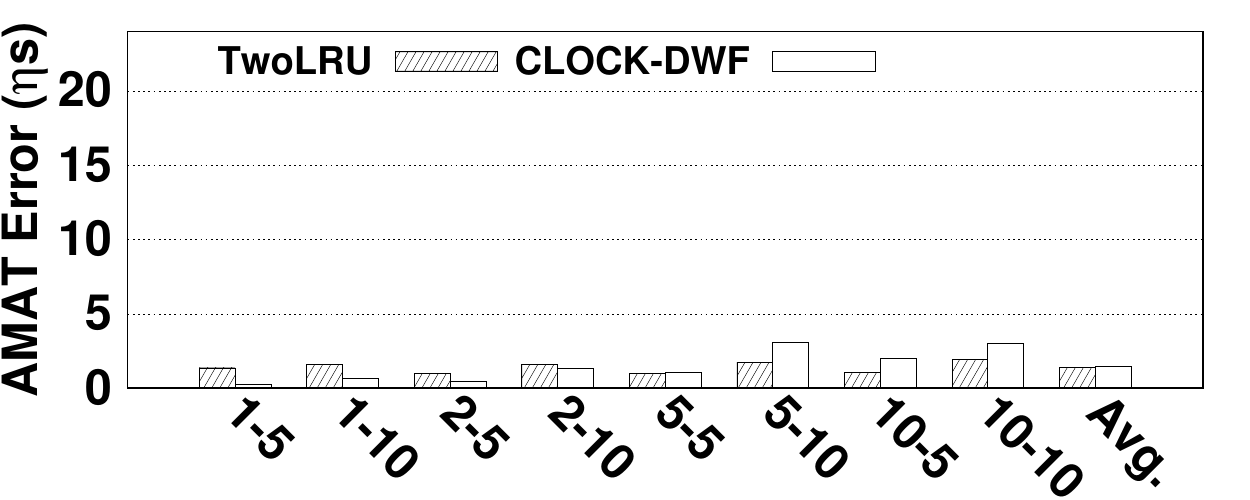}
		\label{fig:cannealerror-lifetime}}
	\hfill
	\subfloat[dedup]{\includegraphics[width=0.242\textwidth]{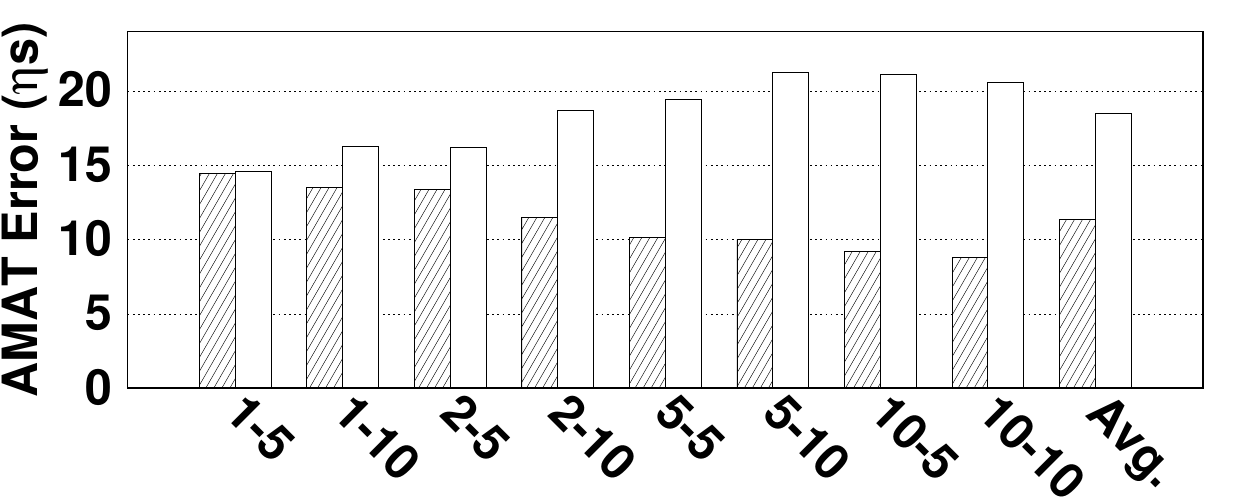}
		\label{fig:deduperror-lifetime}}
	\hfill
	\vspace{-.5cm}
	\subfloat[facesim]{\includegraphics[width=0.242\textwidth]{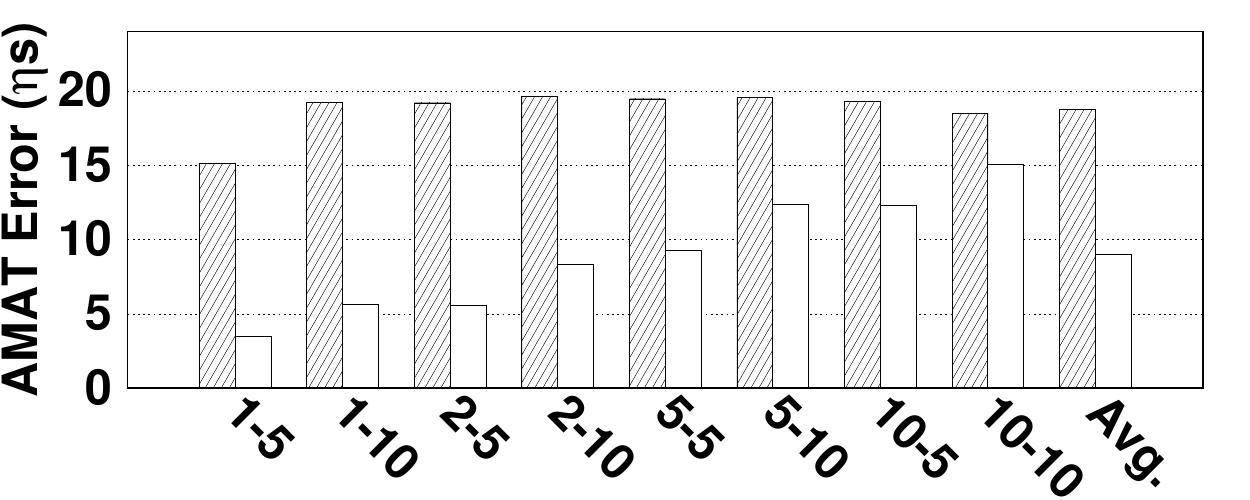}
		\label{fig:facesimerror-lifetime}}
	\hfill
	\subfloat[ferret]{\includegraphics[width=0.242\textwidth]{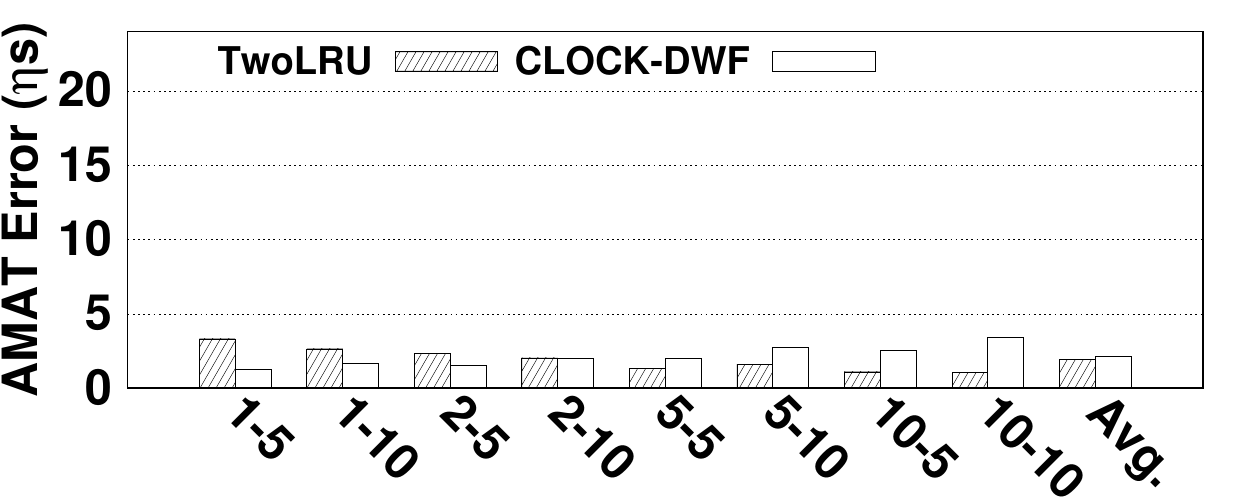}
		\label{fig:ferreterror-lifetime}}
	\hfill
	\subfloat[fluidanimate]{\includegraphics[width=0.242\textwidth]{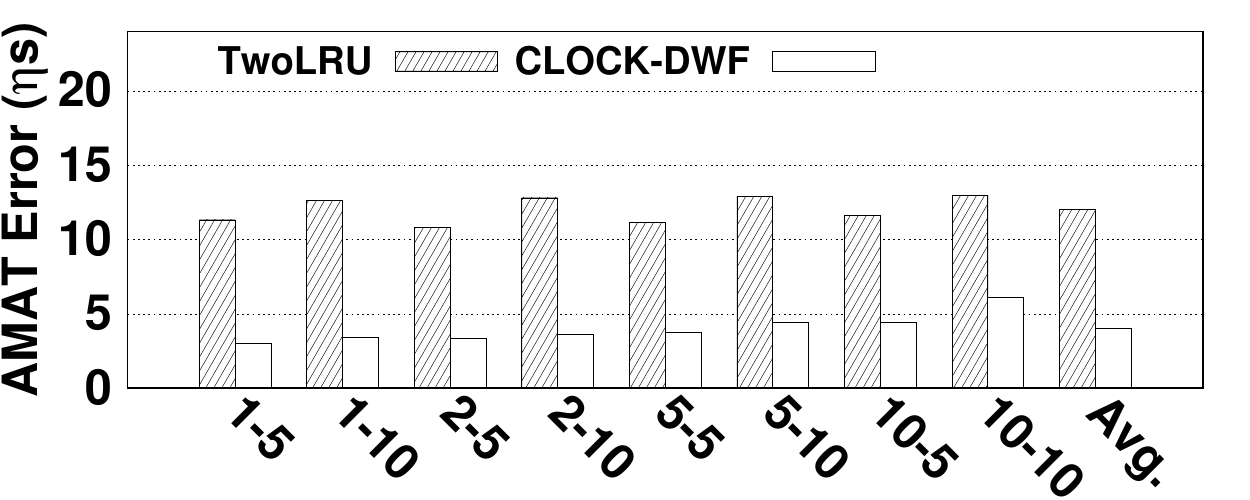}
		\label{fig:fluidanimateerror-lifetime}}
	\hfill
	\subfloat[freqmine]{\includegraphics[width=0.242\textwidth]{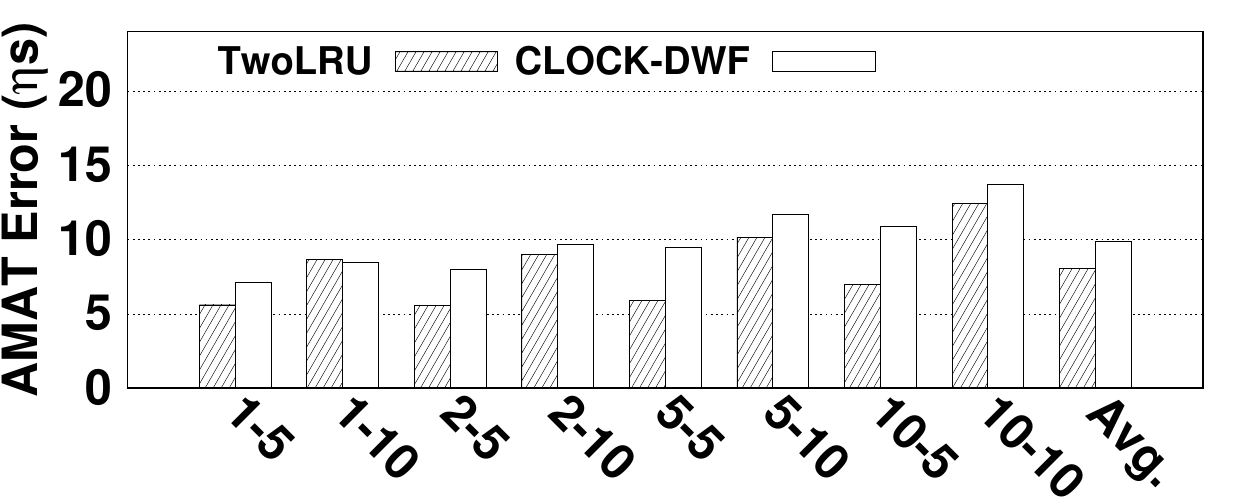}
		\label{fig:freqmineerror-lifetime}}
	\hfill
	\vspace{-.5cm}
	\subfloat[raytrace]{\includegraphics[width=0.242\textwidth]{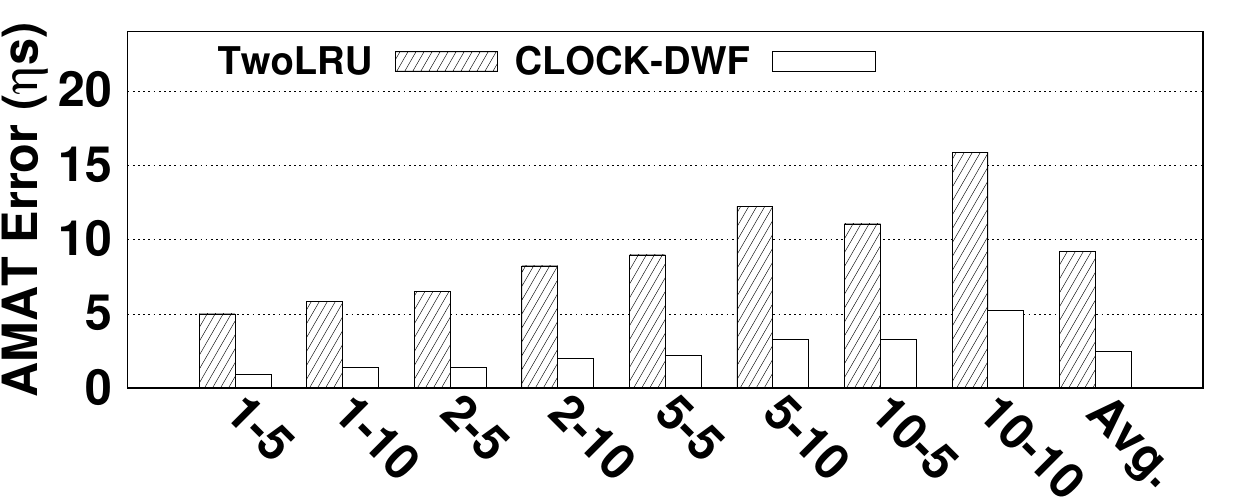}
		\label{fig:raytraceerror-lifetime}}
	\hfill
	\subfloat[streamcluster]{\includegraphics[width=0.242\textwidth]{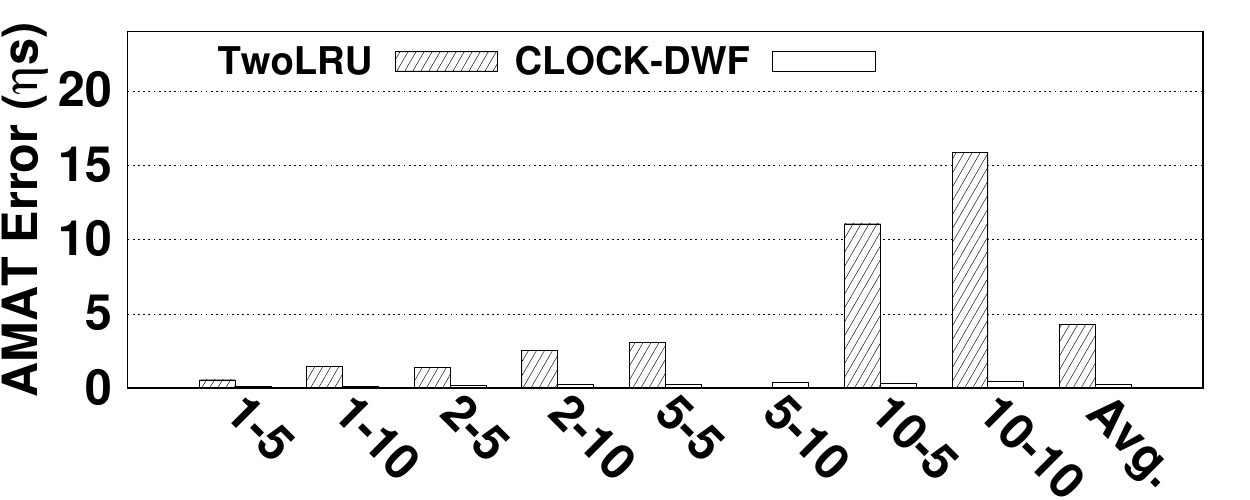}
		\label{fig:streamclustererror-lifetime}}
	\hfill
	\subfloat[vips]{\includegraphics[width=0.242\textwidth]{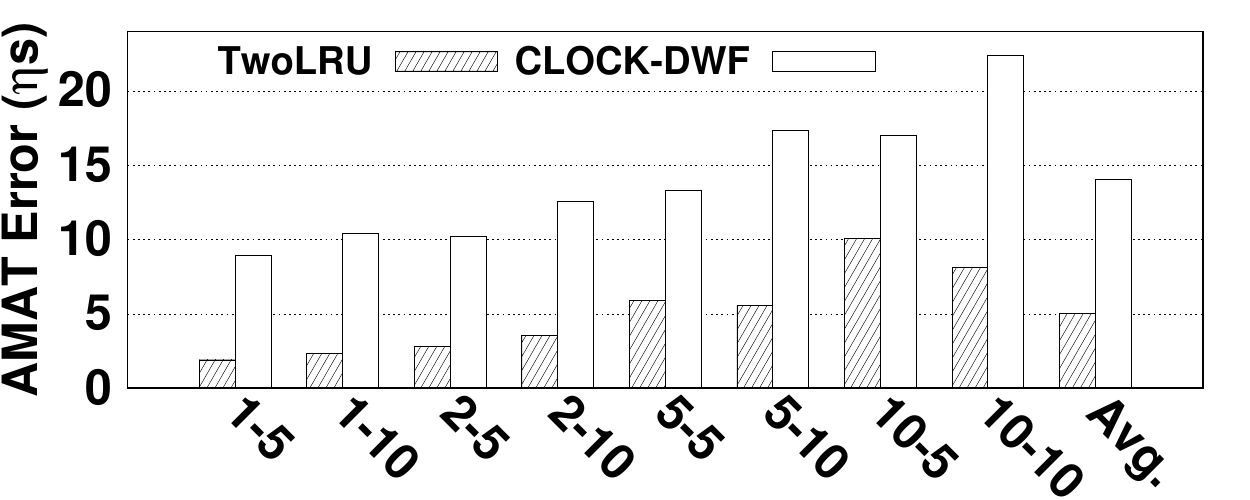}
		\label{fig:vipserror-lifetime}}
	\hfill
	\subfloat[x264]{\includegraphics[width=0.242\textwidth]{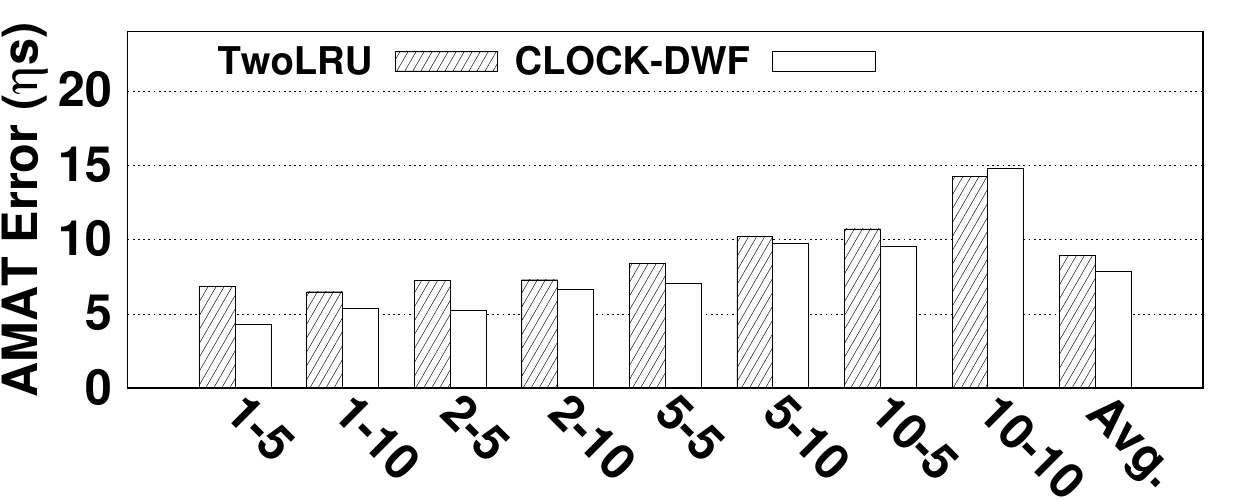}
		\label{fig:x264error-lifetime}}
	\vspace{-.2cm}
	\caption{Absolute Response Time}
	\label{fig:absresponse}
	\vspace{-0.5cm}
\end{figure*}

\begin{figure*}[t]
	\centering
	\subfloat[blackscholes]{\includegraphics[width=0.242\textwidth]{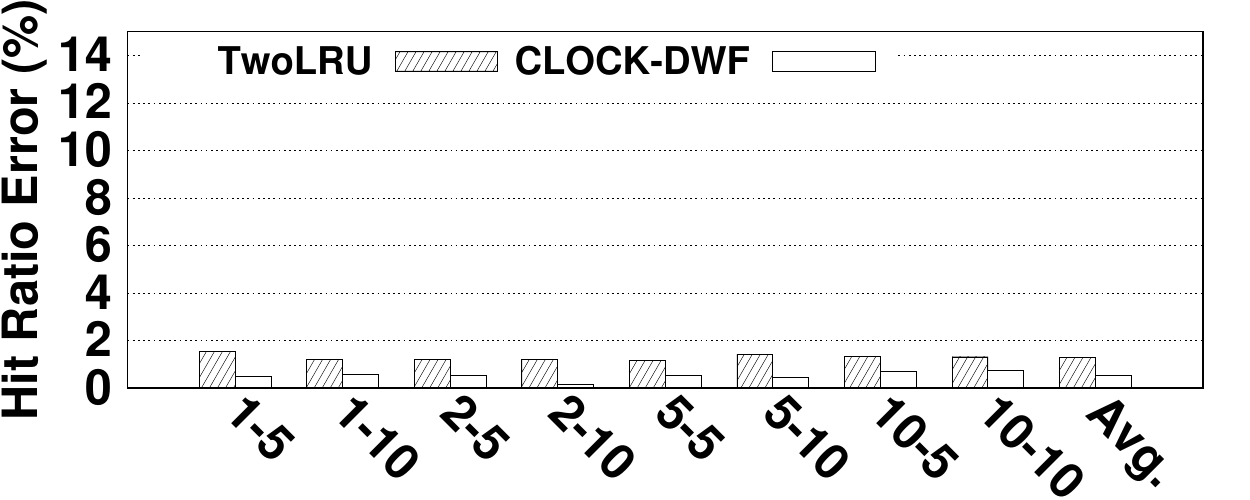}
		\label{fig:blackscholes-lifetime}}
	\hfill
	\subfloat[bodytrack]{\includegraphics[width=0.242\textwidth]{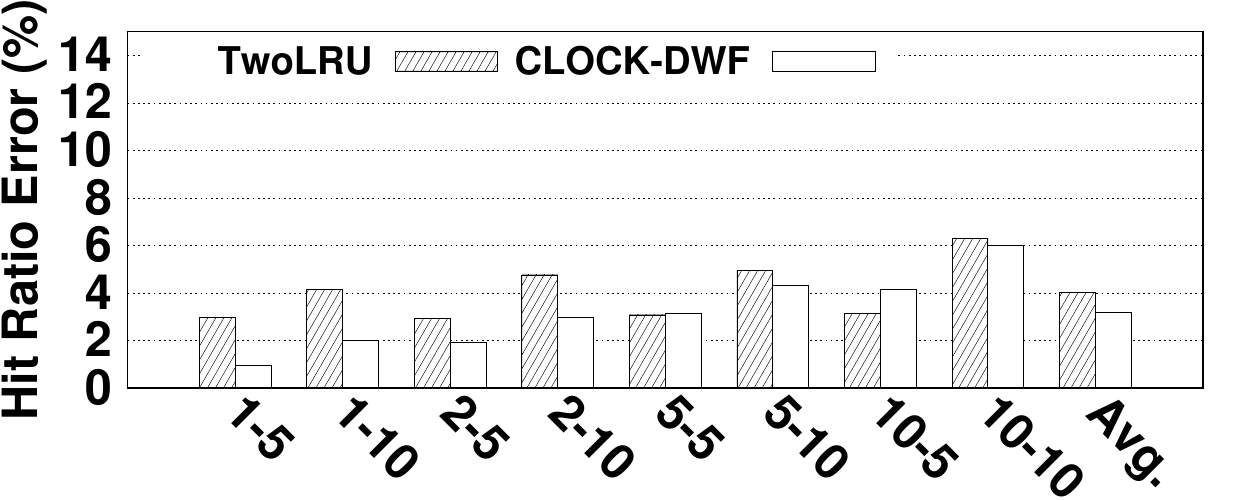}
		\label{fig:bodytrackerror-lifetime}}
	\hfill
	\subfloat[canneal]{\includegraphics[width=0.242\textwidth]{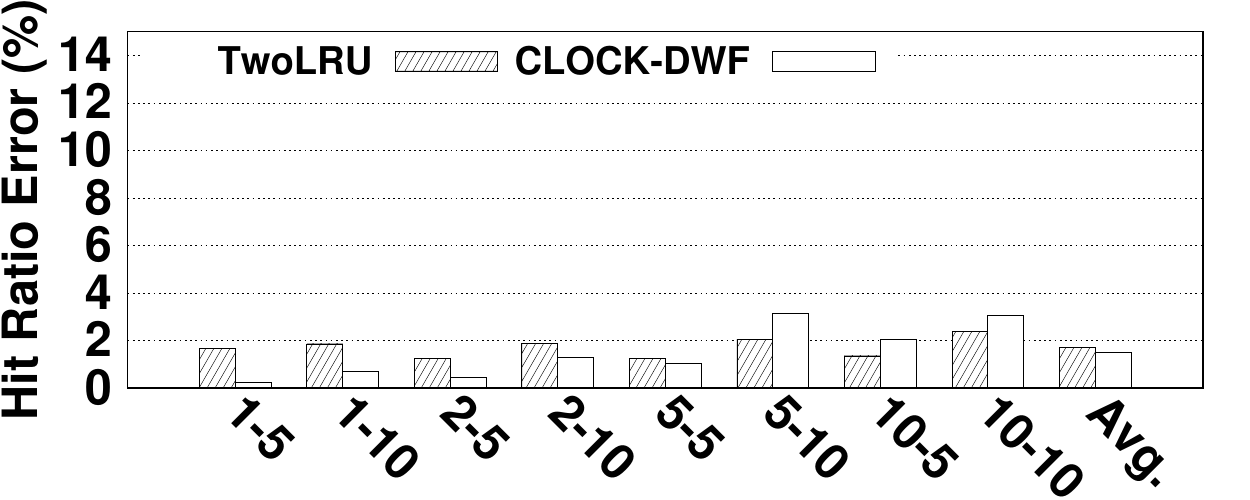}
		\label{fig:cannealerror-lifetime}}
	\hfill
	\subfloat[dedup]{\includegraphics[width=0.242\textwidth]{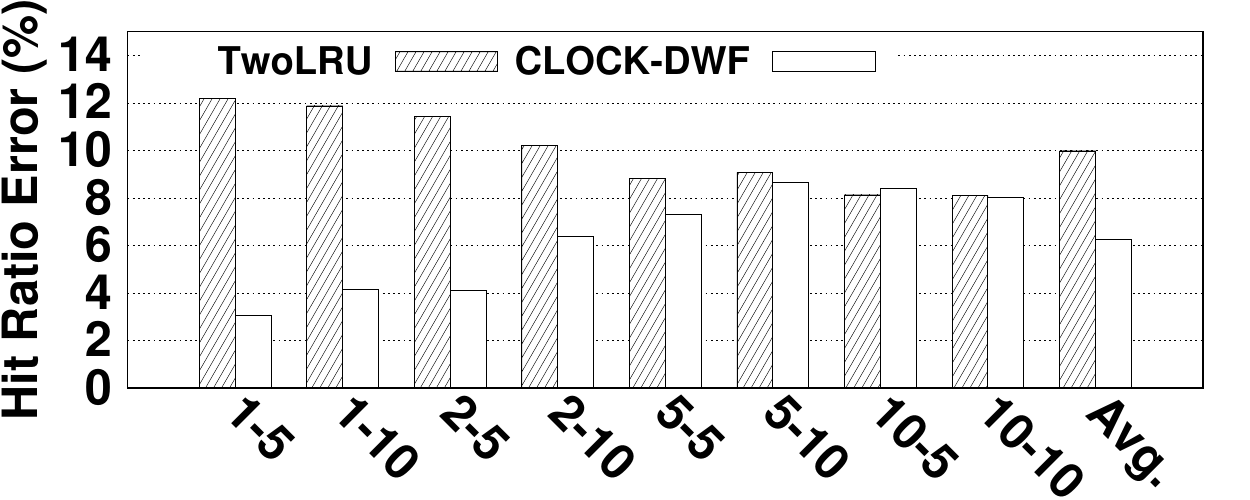}
		\label{fig:deduperror-lifetime}}
	\hfill
	\vspace{-.5cm}
	\subfloat[facesim]{\includegraphics[width=0.242\textwidth]{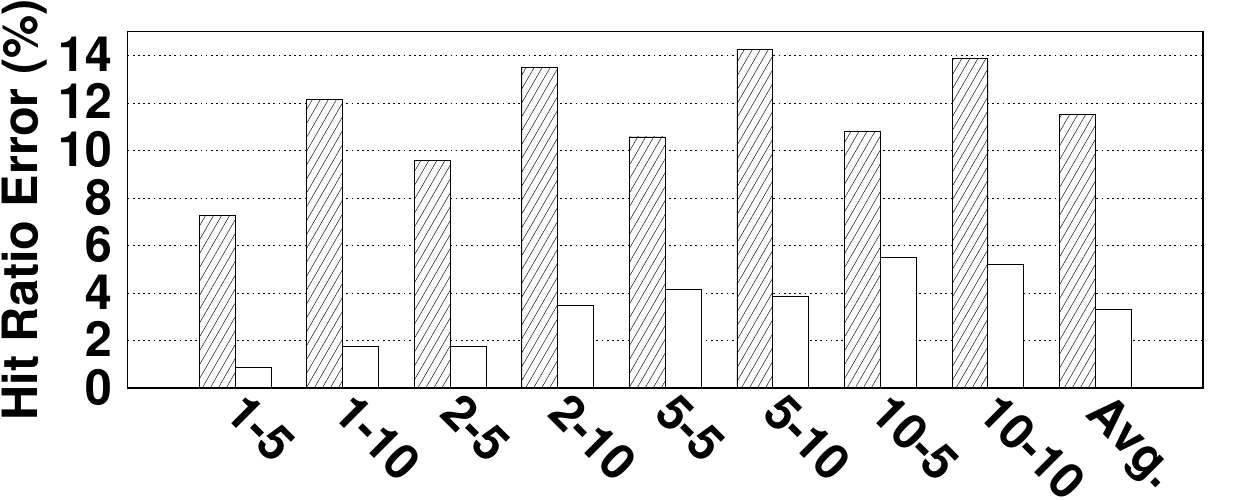}
		\label{fig:facesimerror-lifetime}}
	\hfill
	\subfloat[ferret]{\includegraphics[width=0.242\textwidth]{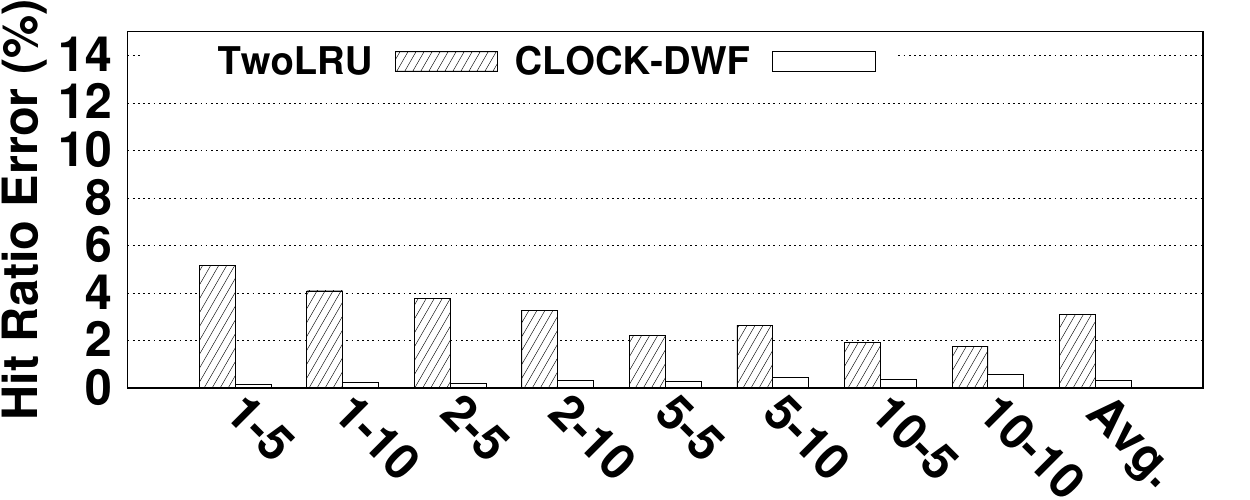}
		\label{fig:ferreterror-lifetime}}
	\hfill
	\subfloat[fluidanimate]{\includegraphics[width=0.242\textwidth]{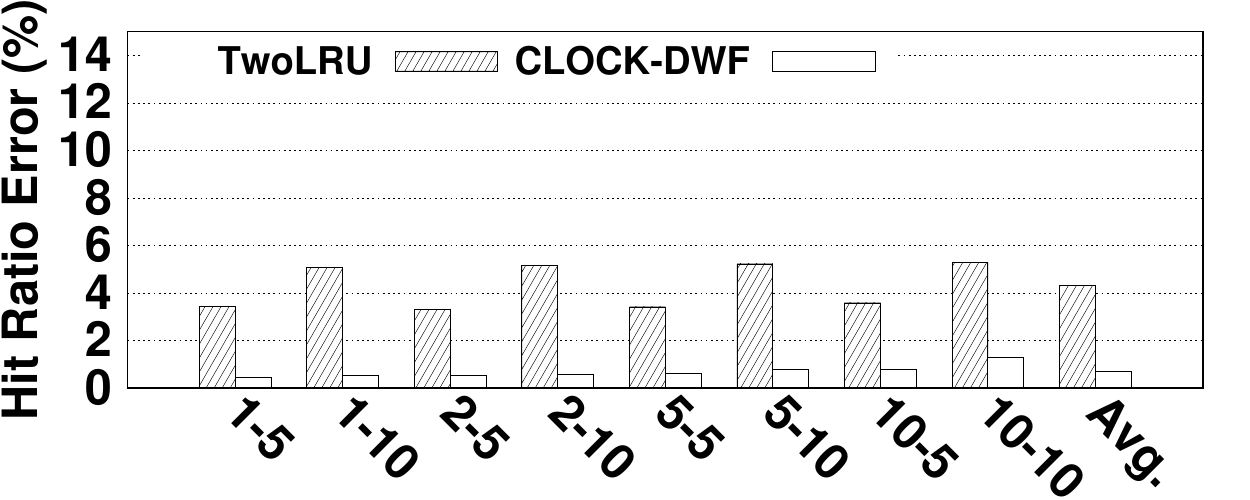}
		\label{fig:fluidanimateerror-lifetime}}
	\hfill
	\subfloat[freqmine]{\includegraphics[width=0.242\textwidth]{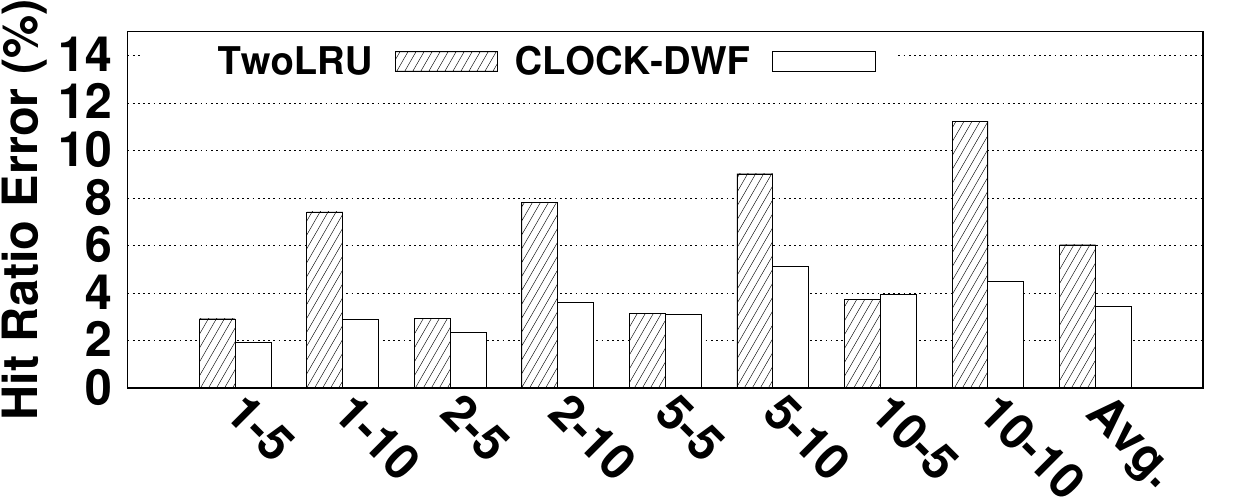}
		\label{fig:freqmineerror-lifetime}}
	\hfill
	\vspace{-.5cm}
	\subfloat[raytrace]{\includegraphics[width=0.242\textwidth]{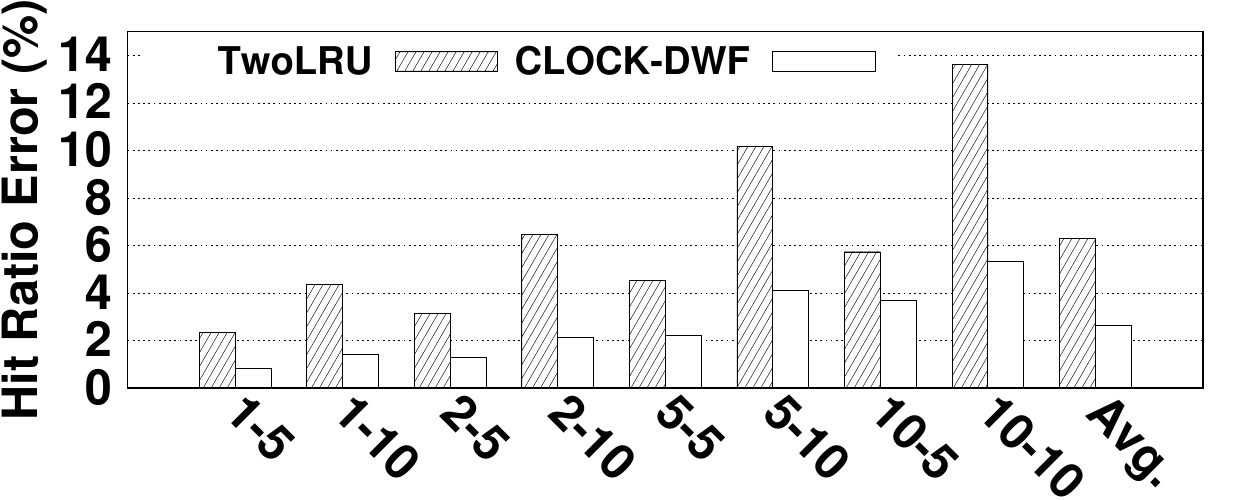}
		\label{fig:raytraceerror-lifetime}}
	\hfill
	\subfloat[streamcluster]{\includegraphics[width=0.242\textwidth]{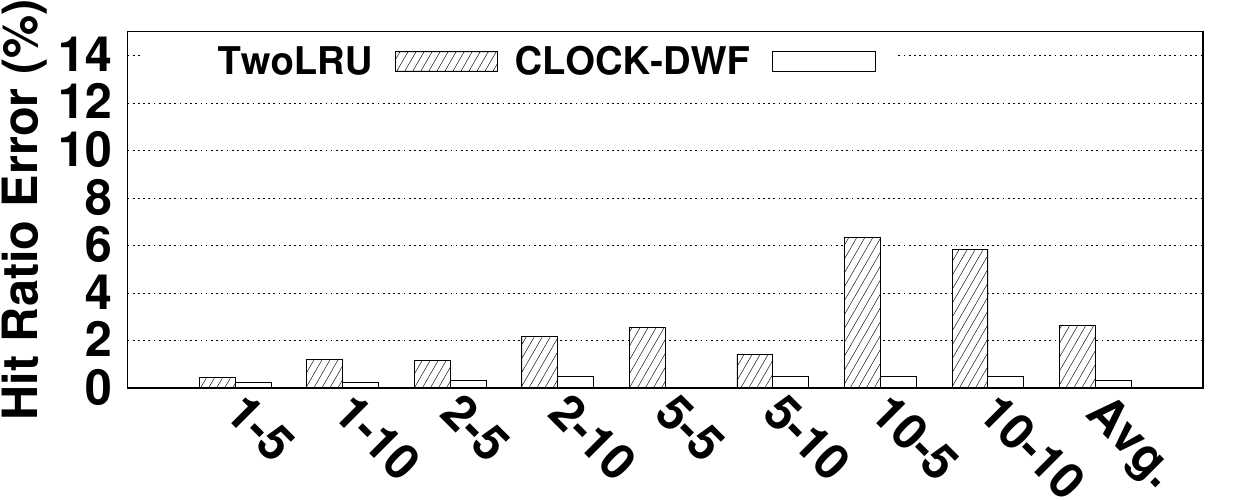}
		\label{fig:streamclustererror-lifetime}}
	\hfill
	\subfloat[vips]{\includegraphics[width=0.242\textwidth]{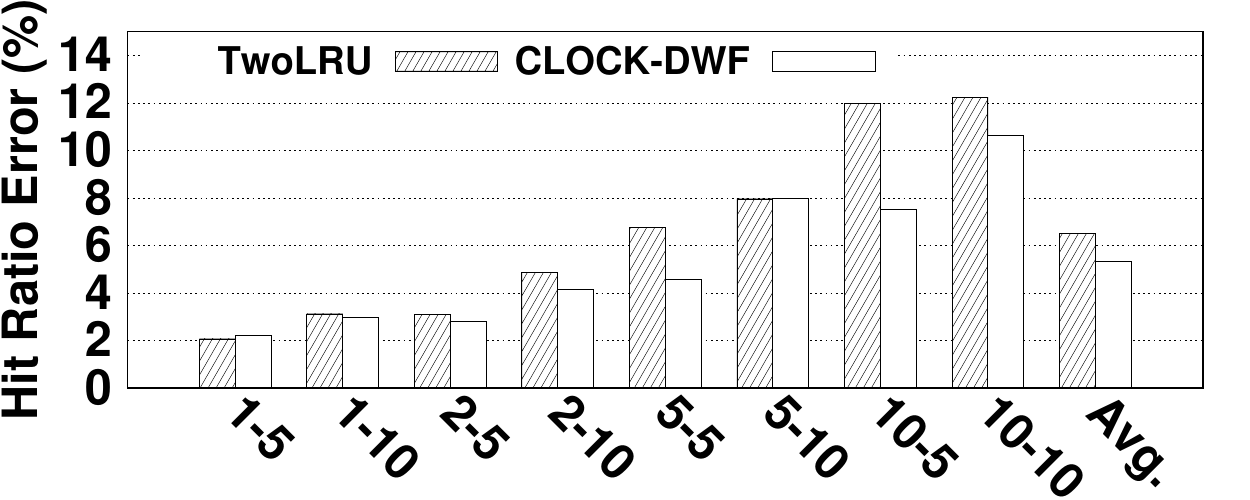}
		\label{fig:vipserror-lifetime}}
	\hfill
	\subfloat[x264]{\includegraphics[width=0.242\textwidth]{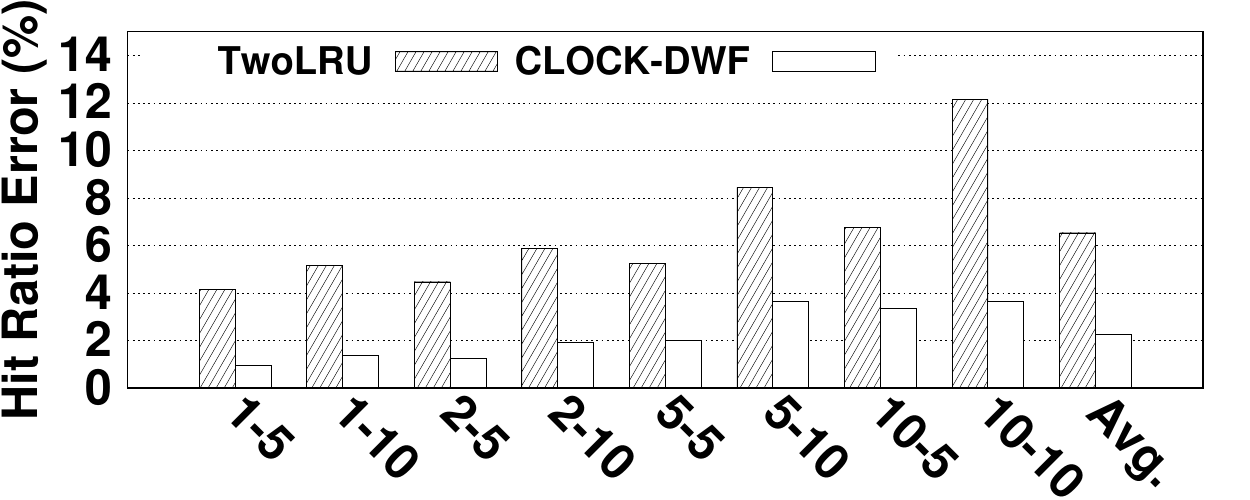}
		\label{fig:x264error-lifetime}}
	\vspace{-.2cm}
	\caption{Absolute Hit Ratio Values}
	\label{fig:abshitratio}
	\vspace{-0.5cm}
\end{figure*}

\subsection{Assumptions}
The HMAs that can be evaluated by the proposed model should have the following criteria based on the definition of HMAs:
\begin{itemize}[leftmargin=*]
	\item Data page eviction probabilities should be only dependent on the corresponding information in \emph{mapping} (Equation \ref{eq:eviction}).
	\item Accessed data pages should have a static predefined mapping information , i.e., the first position of queue in LRU algorithm (denoted as \emph{Hit\_Mapping} in Equation \ref{eq:hitaccess}).
	\item \emph{mapping.NVM} and \emph{mapping.DRAM} should be totally ordered under \emph{less than or equal} ($\leq$) as denoted by Equation \ref{eq:ordered}.
	\item A page can be migrated from NVM to DRAM (promotion) only when it is accessed (Equation \ref{eq:migration}).
	\item Evicted data pages from DRAM should be moved to NVM and as such, in the updated mapping (denoted as NM in Equation \ref{eq:demotion}), they should be treated similar to a hit access in NVM (Equation \ref{eq:demotion}).
	\item Evicted data pages from NVM are removed from memory (Equation \ref{eq:nvmeviction}).
	\item Accessed data page will be assigned the highest position in $mapping$ (Equation \ref{eq:static}).
	%\item Migrations from DRAM to NVM (demotions) are triggered when a new data page enters DRAM.
\end{itemize}

\begin{figure}[h]
	\footnotesize
	\vspace{-.2cm}
	\begin{align}
	\label{eq:eviction}
	EvicP(page) &\propto mapping[page] \nonumber \\
	\forall p \in mapping&: p \neq page \Rightarrow evicP(page) \perp mapping[p]
	\end{align}
	\vspace{-.2cm}
	\begin{align}
	\label{eq:hitaccess}
	\forall mapping,& \forall page : U\!pd(mapping, page, new\_mapping) \nonumber \\
	\Rightarrow &new\_mapping[page] = \text{Hit\_Mapping}
	\end{align}
	\vspace{-.2cm}
	\begin{align}
	\label{eq:ordered}
	&\forall M \in \{D\!R\!A\!M, N\!V\!M\}, \forall P1, P2, P3 \in mapping.M: \nonumber \\
	&(P1 \leq P2 \wedge P2 \leq P1 \Rightarrow P1 = P2)  \wedge 
	(P1 \leq P2 \wedge P2 \leq P3 \Rightarrow  \nonumber \\ 
	& P1 \leq P3) \wedge (P1 \leq P2 \vee P2 \leq P1)
	\end{align}
	\vspace{-.2cm}
	\begin{align}
	\label{eq:migration}
	U\!pd(mapping,& page, new\_mapping) \wedge mig(mapping, mig\_page) \nonumber \\
	\Rightarrow &mig\_page = N\!U\!L\!L \vee mig\_page = page
	\end{align}
	\vspace{-.2cm}
	\begin{align}
	\label{eq:demotion}
	&P \in D\!R\!A\!M \wedge U\!pd(M, P2, N\!M) \wedge eviction\_victim = P2 \nonumber \\
	&\Rightarrow N\!M[P] = \text{Hit\_Mapping} \wedge P \in N\!M.N\!V\!M
	\end{align}
	\vspace{-.2cm}
	\begin{align}
	\label{eq:nvmeviction}
	&P \in N\!V\!M \wedge Upd(M, P2, N\!M) \wedge eviction\_victim = P\nonumber \\
	&\Rightarrow P \not\in N\!M
	\end{align}
	\vspace{-.2cm}
	\begin{align}
	\label{eq:static}
	& \forall M \in \{D\!R\!A\!M, N\!V\!M\}, \forall p \in {mapping}.M : p \leq \text{Hit\_Mapping}
	\end{align}
	\vspace{-.5cm}
\end{figure}

\vspace{-.3cm}
\section{Absolute Error Values}
\label{sec:asberror}
Here, absolute error values for hit ratio and AMAT are reported.
Relative errors for both hit ratio and AMAT are presented in Section 6.2.%\ref{sec:accuracy}
The absolute error of AMAT for various benchmarks is 7.14\ $\eta s$ on average which is reported in Fig. \ref{fig:absresponse}.
The maximum absolute error for estimating AMAT belongs to \emph{vips} benchmark in CLOCK-DWF which is 22.35 $\eta s$.
In \emph{bodytrack} benchmark, TwoLRU and CLOCK-DWF have almost the same relative AMAT error as depicted in Fig. 14
while the absolute AMAT error is almost twofold in CLOCK-DWF.
This is due to the difference in number of disks and memory accesses in two examined HMAs.%\ref{fig:totalerrorperf}

The average hit ratio error is 5.31\% and 2.48\% for TwoLRU and CLOCK-DWF, respectively as demonstrated in Fig. \ref{fig:abshitratio}.
The \emph{dedup} benchmark has highest absolute hit ratio error (8.11\% on average) in both examined HMAs which is due to the anomalies in the access distribution of this benchmark.
Such anomaly also exists in estimating AMAT and NVM lifetime of \emph{dedup} benchmark.
The highest hit ratio absolute error, however, belongs to \emph{facesim} benchmark in TwoLRU which is 14.2\%.
CLOCK-DWF has a lower maximum hit ratio error of 10.6\% which belongs to \emph{vips} benchmark.
\end{document}
